# Supplementary material for: Discriminative Adversarial Privacy: Balancing Accuracy and Membership Privacy in Neural Networks
Source: arXiv:2306.03054 source file (2023-06-05)
Supplement: Supplementary file 1 [file supplementary.tex]

\newpage
\section*{AOP $\lambda$ Analysis}
This section presents the Accuracy Over Privacy (AOP) results for different values of lambda ($\lambda$), distinct from those utilized in the primary paper. Specifically, Tables~\ref{table:aop1},~\ref{table:aop5},~\ref{table:aop10} display the AOP metric outcomes for lambda values of 1, 5, and 10, respectively.
Table~\ref{table:aop1} stands out as the only one displaying accuracy and Area Under the Curve (AUC) of the Membership Inference Attack (MIA) at equivalent magnitudes. In this particular scenario, it is evident that the trade-off between these two metrics exclusively favors the Reg model, followed by the DAP models, compared to the Baseline model.
As the $\lambda$ value increases, the AOP scores decrease, indicating a greater penalty in proportion to the AUC. Both Table~\ref{table:aop5} and Table~\ref{table:aop10} demonstrate how the average AOP of the Baseline diminishes at a much faster rate than that of the other models. Particularly in Table~\ref{table:aop10}, the DAP models indisputably emerge as the optimal choice for managing the trade-off, trailed by the DP models, and as a last resort, the Reg model, which exhibits performance very similar to the Baseline model.
It is important to note that DP results tend to deteriorate less than Baseline and Reg results, in many cases surpassing them, as $\lambda$ increases. They do, however, suffer from problems with many classes, an indication of the poor accuracy achieved despite the guaranteed privacy.

\begin{table}[!h]
    \caption{The AOP metric on the test sets ($\lambda=1$). Results improving the baseline are coloured in \textcolor{tabG}{green}, while results worse than the baseline are \textcolor{tabR}{red}. The best results among them are in \textbf{bold}, while the second best are \underline{underlined}.}
    \centering 
    \resizebox{\textwidth}{!}{%
    \begin{tabularx}{\textwidth}{| l || c | Y c Y Y Y Y Y |}
    \hline
      \textbf{Dataset} & \textbf{Baseline} & \textbf{Reg}  & \textbf{${\epsilon=0.5}$} & \textbf{${\epsilon=1}$}  & \textbf{${\epsilon=2}$}  & \textbf{${\epsilon=4}$}  & \textbf{DAP$_t$}  & \textbf{DAP$_v$}\\
    \hline \hline
    \textbf{Cifar-10} & 0.605 &	\textbf{\textcolor{tabG}{0.643}} &	\textcolor{tabR}{0.310} &	\textcolor{tabR}{0.355} & \textcolor{tabR}{0.402} & \textcolor{tabR}{0.415}	& \textcolor{tabG}{\underline{0.615}} &	\textcolor{tabG}{0.607}\\
    \textbf{Cifar-100} & 0.399	&\textbf{\textcolor{tabG}{0.428}}	&\textcolor{tabR}{0.039}	&\textcolor{tabR}{0.080}	&\textcolor{tabR}{0.089}	&\textcolor{tabR}{0.071}&	\textcolor{tabR}{\underline{0.305}}	& \textcolor{tabR}{0.273}\\
    \textbf{FMNIST} & 0.844	& \textcolor{tabR}{0.824} & \textcolor{tabR}{0.603}& \textcolor{tabR}{0.698}& \textcolor{tabR}{0.730} &	\textcolor{tabR}{0.766} &	\textcolor{tabG}{\underline{0.854}} & \textcolor{tabG}{\textbf{0.861}} \\
    \textbf{EuroSAT} & 0.880	& \textbf{\textcolor{tabG}{0.900}}	& \textcolor{tabR}{0.305}	& \textcolor{tabR}{0.586} &\textcolor{tabR}{0.681} & \textcolor{tabR}{0.643} 	& \textcolor{tabG}{\underline{0.898}} &	\textcolor{tabG}{0.891} \\
    \textbf{TinyImagenet} & 0.303 &	\textbf{\textcolor{tabG}{0.319}} &	\textcolor{tabR}{0.030} &	\textcolor{tabR}{0.032} &	\textcolor{tabR}{0.031} &	\textcolor{tabR}{0.025} &	\textcolor{tabR}{\underline{0.252}}& \textcolor{tabR}{0.213}\\
    \textbf{OxfordFlowers} & 0.372 & \textcolor{tabG}{\textbf{0.431}} &	\textcolor{tabR}{0.028} &	\textcolor{tabR}{0.047} &	\textcolor{tabR}{0.083} &	\textcolor{tabR}{0.131} &	\textcolor{tabR}{\underline{0.269}} &	\textcolor{tabR}{0.247} \\
    \textbf{STL-10} & 0.542 &	\textbf{\textcolor{tabG}{0.577}} &	\textcolor{tabR}{0.084} &	\textcolor{tabR}{0.135} & \textcolor{tabR}{0.247} & \textcolor{tabR}{0.288} &	\textcolor{tabR}{\underline{0.472}}& \textcolor{tabR}{0.379} \\
    \textbf{Cinic-10} & 0.588 & \textcolor{tabR}{\underline{0.577}} & \textcolor{tabR}{0.279} &	\textcolor{tabR}{0.339} & \textcolor{tabR}{0.389} &	\textcolor{tabR}{0.402} &	\textcolor{tabR}{0.565}	& \textcolor{tabR}{\textbf{0.578}}\\
    \hline
    \textbf{Average} & 0.567 & \textbf{\textcolor{tabG}{0.587}} & \textcolor{tabR}{0.210} &	\textcolor{tabR}{0.284} &	\textcolor{tabR}{0.331} & \textcolor{tabR}{0.343}  & \textcolor{tabR}{\underline{0.529}} & \textcolor{tabR}{0.506}\\
    \hline
    \end{tabularx}}%
    \label{table:aop1}
\end{table}
\begin{table}[!h]
    \caption{The AOP metric on the test sets ($\lambda=5$). Results improving the baseline are coloured in \textcolor{tabG}{green}, while results worse than the baseline are \textcolor{tabR}{red}. The best results among them are in \textbf{bold}, while the second best are \underline{underlined}.}
    \centering 
    \resizebox{\textwidth}{!}{%
    \begin{tabularx}{\textwidth}{| l || c | Y c Y Y Y Y Y |}
    \hline
      \textbf{Dataset} & \textbf{Baseline} & \textbf{Reg}  & \textbf{${\epsilon=0.5}$} & \textbf{${\epsilon=1}$}  & \textbf{${\epsilon=2}$}  & \textbf{${\epsilon=4}$}  & \textbf{DAP$_t$}  & \textbf{DAP$_v$}\\
    \hline \hline
    \textbf{Cifar-10} & 0.214 &	\textcolor{tabG}{0.253} &	\textcolor{tabG}{0.298} &	\textcolor{tabG}{0.290} & \textcolor{tabG}{0.346} & \textcolor{tabG}{0.406}	& \textcolor{tabG}{\underline{0.582}} &	\textcolor{tabG}{\textbf{0.583}}\\
    \textbf{Cifar-100} & 0.188	& \textcolor{tabR}{0.180}	&\textcolor{tabR}{0.039}	&\textcolor{tabR}{0.072}	&\textcolor{tabR}{0.084}	&\textcolor{tabR}{0.068}&	\textcolor{tabG}{\textbf{0.269}}	& \textcolor{tabG}{\underline{0.260}}\\
    \textbf{FMNIST} & 0.568	& \textcolor{tabR}{0.516} & \textcolor{tabG}{0.593}& \textcolor{tabG}{0.687}& \textcolor{tabG}{0.707} &	\textcolor{tabG}{0.736} &	\textcolor{tabG}{\underline{0.808}} & \textcolor{tabG}{\textbf{0.821}} \\
    \textbf{EuroSAT} & 0.629	& \textcolor{tabG}{0.723}	& \textcolor{tabR}{0.293}	& \textcolor{tabR}{0.276} &\textcolor{tabG}{0.681} & \textcolor{tabG}{0.633} 	& \textbf{\textcolor{tabG}{0.891}} &	\textcolor{tabG}{\underline{0.884}} \\
    \textbf{TinyImagenet} & 0.143 &	\textcolor{tabG}{0.162} &	\textcolor{tabR}{0.027} &	\textcolor{tabR}{0.032} &	\textcolor{tabR}{0.026} &	\textcolor{tabR}{0.024} &	\textcolor{tabG}{\textbf{0.222}}& \textcolor{tabG}{\underline{0.198}}\\
    \textbf{OxfordFlowers} & 0.069 & \textcolor{tabG}{0.079} &	\textcolor{tabR}{0.020} &	\textcolor{tabR}{0.036} &	\textcolor{tabR}{0.067} &	\textcolor{tabG}{0.102} &	\textcolor{tabG}{\underline{0.201}} &	\textbf{\textcolor{tabG}{0.209}} \\
    \textbf{STL-10} & 0.255 &	\textcolor{tabG}{0.359} &	\textcolor{tabR}{0.082} &	\textcolor{tabR}{0.112} & \textcolor{tabR}{0.238} & \textcolor{tabG}{0.286} &	\textcolor{tabG}{\textbf{0.443}}& \textcolor{tabR}{\underline{0.362}} \\
    \textbf{Cinic-10} & 0.343 & \textcolor{tabR}{0.254} & \textcolor{tabR}{0.277} &	\textcolor{tabR}{0.331} & \textcolor{tabG}{0.379} &	\textcolor{tabG}{0.389} &	\textcolor{tabG}{\underline{0.517}}	& \textcolor{tabG}{\textbf{0.547}}\\
    \hline
    \textbf{Average} & 0.301 & \textcolor{tabG}{0.316} & \textcolor{tabR}{0.204} &	\textcolor{tabR}{0.267} &	\textcolor{tabG}{0.316} & \textcolor{tabG}{0.331}  & \textbf{\textcolor{tabG}{0.492}} & \textcolor{tabG}{\underline{0.483}}\\
    \hline
    \end{tabularx}}%
    \label{table:aop5}
\end{table}
\begin{table}[!h]
    \caption{The AOP metric on the test sets ($\lambda=10$). Results improving the baseline are coloured in \textcolor{tabG}{green}, while results worse than the baseline are \textcolor{tabR}{red}. The best results among them are in \textbf{bold}, while the second best are \underline{underlined}.}
    \centering 
    \resizebox{\textwidth}{!}{%
    \begin{tabularx}{\textwidth}{| l || c | Y c Y Y Y Y Y |}
    \hline
      \textbf{Dataset} & \textbf{Baseline} & \textbf{Reg}  & \textbf{${\epsilon=0.5}$} & \textbf{${\epsilon=1}$}  & \textbf{${\epsilon=2}$}  & \textbf{${\epsilon=4}$}  & \textbf{DAP$_t$}  & \textbf{DAP$_v$}\\
    \hline \hline
    \textbf{Cifar-10} & 0.059 &	\textcolor{tabG}{0.079} &	\textcolor{tabG}{0.283} &	\textcolor{tabG}{0.225} & \textcolor{tabG}{0.287} & \textcolor{tabG}{0.394}	& \textcolor{tabG}{\underline{0.543}} &	\textcolor{tabG}{\textbf{0.555}}\\
    \textbf{Cifar-100} & 0.074	& \textcolor{tabR}{0.061}	&\textcolor{tabR}{0.039}	&\textcolor{tabR}{0.062}	&\textcolor{tabG}{0.078}	&\textcolor{tabR}{0.064}&	\textcolor{tabG}{\underline{0.230}}	& \textcolor{tabG}{\textbf{0.245}}\\
    \textbf{FMNIST} & 0.346	& \textcolor{tabR}{0.288} & \textcolor{tabG}{0.581}& \textcolor{tabG}{0.674}& \textcolor{tabG}{0.680} &	\textcolor{tabG}{0.701} &	\textcolor{tabG}{\underline{0.754}} & \textcolor{tabG}{\textbf{0.773}} \\
    \textbf{EuroSAT} & 0.412	& \textcolor{tabG}{0.551}	& \textcolor{tabR}{0.279}	& \textcolor{tabG}{0.565} &\textcolor{tabG}{0.681} & \textcolor{tabG}{0.621} 	& \textcolor{tabG}{\underline{0.882}} &	\textcolor{tabG}{\textbf{0.875}} \\
    \textbf{TinyImagenet} & 0.056 &	\textcolor{tabG}{0.069} &	\textcolor{tabR}{0.023} &	\textcolor{tabR}{0.031} &	\textcolor{tabR}{0.021} &	\textcolor{tabR}{0.023} &	\textcolor{tabG}{\textbf{0.190}}& \textcolor{tabG}{\underline{0.181}}\\
    \textbf{OxfordFlowers} & 0.008 & \textcolor{tabG}{0.009} &	\textcolor{tabG}{0.014} &	\textcolor{tabG}{0.025} &	\textcolor{tabG}{0.052} &	\textcolor{tabG}{0.075} &	\textcolor{tabG}{\underline{0.269}} &	\textcolor{tabG}{\textbf{0.247}} \\
    \textbf{STL-10} & 0.099 &	\textcolor{tabG}{0.198} &	\textcolor{tabR}{0.081} &	\textcolor{tabR}{0.089} & \textcolor{tabG}{0.226} & \textcolor{tabG}{0.283} &	\textcolor{tabG}{\textbf{0.409}}& \textcolor{tabG}{\underline{0.341}} \\
    \textbf{Cinic-10} & 0.175 & \textcolor{tabR}{0.091} & \textcolor{tabG}{0.274} &	\textcolor{tabG}{0.321} & \textcolor{tabG}{0.368} &	\textcolor{tabG}{0.374} &	\textcolor{tabG}{\underline{0.464}}	& \textcolor{tabG}{\textbf{0.510}}\\
    \hline
    \textbf{Average} & 0.154 & \textcolor{tabG}{0.168} & \textcolor{tabG}{0.197} &	\textcolor{tabG}{0.249} &	\textcolor{tabG}{0.299} & \textcolor{tabG}{0.317}  & \textcolor{tabG}{\underline{0.451}} & \textcolor{tabG}{\textbf{0.456}}\\
    \hline
    \end{tabularx}}%
    \label{table:aop10}
    % \vspace{-10pt}
\end{table}

\newpage
\section*{MIA Against Slices}
The effectiveness of Membership Inference Attacks (MIAs) relies on whether they target correctly classified samples from the attacked model or not. This assertion is precisely demonstrated in Table~\ref{table:miss} and Table~\ref{table:ok}.
In Table~\ref{table:miss}, showing the results of the MIA attack against the miss-classified slices, the Baseline and Reg models are particularly vulnerable, while the DP models exhibit high levels of security. The DAP technique achieves results close to random guessing, thus ensuring strong protection.
On the other hand, Table~\ref{table:ok} reveals the poor performance of MIAs on correctly classified samples on average. Moreover, both the Baseline and Reg models enable the attacking model to achieve an AUC close to 0.5, which, in many cases, surpasses the AUC obtained by the DP models. This suggests that correctly predicted test set samples possess similar characteristics to the training data, making them challenging to distinguish.
However, the most noteworthy result is observed in the DAP models. They not only outperform the Baseline model but also emerge as the overall best, surpassing even the DP models.
\begin{table}[!h]
    \caption{The AUC metric of the MIAs over the wrongly classified samples. Results improving the baseline are coloured in \textcolor{tabG}{green}, while results worse than the baseline are \textcolor{tabR}{red}. The best results among them are in \textbf{bold}, while the second best are \underline{underlined}.}
    \centering 
    \resizebox{\textwidth}{!}{%
    \begin{tabularx}{\textwidth}{| l || c | Y c Y Y Y Y Y |}
    \hline
    \textbf{Dataset} & \textbf{Baseline} & \textbf{Reg}  & \textbf{${\epsilon=0.5}$} & \textbf{${\epsilon=1}$}  & \textbf{${\epsilon=2}$}  & \textbf{${\epsilon=4}$}  & \textbf{DAP$_t$}  & \textbf{DAP$_v$}\\
    \hline \hline
    \textbf{Cifar-10} & 0.753 & \textcolor{tabG}{0.689} & \underline{\textcolor{tabG}{0.505}} & \textbf{\textcolor{tabG}{0.503}} & \textbf{\textcolor{tabG}{0.503}} & \textcolor{tabG}{0.506} & \textcolor{tabG}{0.510} & \underline{\textcolor{tabG}{0.505}}\\
    \textbf{Cifar-100} & 0.610 & \textcolor{tabR}{0.627} & \textbf{\textcolor{tabG}{0.501}} & \textcolor{tabG}{0.506} & \textcolor{tabG}{0.538} & \underline{\textcolor{tabG}{0.505}} & \textcolor{tabG}{0.518} & \textcolor{tabG}{0.509}\\
    \textbf{FMNIST} & 0.659 & \textcolor{tabR}{0.768} & \underline{\textcolor{tabG}{0.502}} & \textcolor{tabG}{0.506} & \underline{\textcolor{tabG}{0.502}} & \textbf{\textcolor{tabG}{0.500}} & \textcolor{tabG}{0.523} & \textcolor{tabG}{0.527} \\
    \textbf{EuroSAT} & 0.698 & \textcolor{tabG}{0.563} & \textbf{\textcolor{tabG}{0.500}} & \underline{\textcolor{tabG}{0.501}} & \textcolor{tabG}{0.523} & \textcolor{tabG}{0.504} & \textcolor{tabG}{0.527} & \textcolor{tabG}{0.528}\\
    \textbf{TinyImagenet} & 0.585 & \textcolor{tabG}{0.565} & \textcolor{tabG}{0.504} & \underline{\textcolor{tabG}{0.502}} & \textbf{\textcolor{tabG}{0.501}} & \textcolor{tabG}{0.505} & \textcolor{tabG}{0.518} & \textcolor{tabG}{0.508}\\
    \textbf{OxfordFlowers} & 0.785 & \textcolor{tabR}{0.837} & \underline{\textcolor{tabG}{0.529}} & \textcolor{tabG}{0.555} & \textbf{\textcolor{tabG}{0.518}} & \textcolor{tabG}{0.532} & \textcolor{tabG}{0.547} & \textcolor{tabG}{0.537}\\
    \textbf{STL-10} & 0.636 & \textcolor{tabG}{0.567} & \textbf{\textcolor{tabG}{0.500}} & \textcolor{tabG}{0.506} & \textcolor{tabG}{0.506} & \underline{\textcolor{tabG}{0.504}} & \textcolor{tabG}{0.509} & \underline{\textcolor{tabG}{0.504}}\\
    \textbf{Cinic-10} & 0.560 & \textcolor{tabR}{0.649} & \textbf{\textcolor{tabG}{0.501}} & \textcolor{tabG}{0.503} & \textcolor{tabG}{0.503} & \underline{\textcolor{tabG}{0.502}} & \textcolor{tabG}{0.508} & \textcolor{tabG}{0.510}\\
    \hline
    \textbf{Average} & 0.661 & \textcolor{tabG}{0.658} & \textbf{\textcolor{tabG}{0.505}} & \textcolor{tabG}{0.510} & \textcolor{tabG}{0.512} & \textcolor{tabG}{\underline{0.507}} & \textcolor{tabG}{0.520} & \textcolor{tabG}{0.516}\\
    \hline
    \end{tabularx}}%
    \label{table:miss}
\end{table}

\begin{table}[!h]
    \caption{The AUC metric of the MIAs over the correctly classified samples. Results improving the baseline are coloured in \textcolor{tabG}{green}, while results worse than the baseline are \textcolor{tabR}{red}. The best results among them are in \textbf{bold}, while the second best are \underline{underlined}.}
    \centering 
    \resizebox{\textwidth}{!}{%
    \begin{tabularx}{\textwidth}{| l || c | Y c Y Y Y Y Y |}
    \hline
    \textbf{Dataset} & \textbf{Baseline} & \textbf{Reg}  & \textbf{$\epsilon=0.5$} & \textbf{$\epsilon=1$}  & \textbf{ $\epsilon=2$}  & \textbf{$\epsilon=4$}  & \textbf{DAP$_t$}  & \textbf{DAP$_v$}\\
    \hline \hline
    \textbf{Cifar-10} & 0.545 & \textcolor{tabG}{0.537} & \textbf{\textcolor{tabG}{0.500}} & \textcolor{tabG}{\underline{0.502}} & \textcolor{tabG}{0.503} & \textcolor{tabG}{0.506} & \textcolor{tabG}{0.507} & \textcolor{tabG}{0.504} \\
    \textbf{Cifar-100} & 0.516 & \textcolor{tabR}{0.517} & \textcolor{tabG}{0.512} & \textcolor{tabR}{0.521} & \textcolor{tabG}{\underline{0.508}} & \textcolor{tabG}{0.511} & \textbf{\textcolor{tabG}{0.507}} & \textcolor{tabG}{0.509}\\
    \textbf{FMNIST} & 0.514 & \textcolor{tabR}{0.532} & \textcolor{tabG}{\underline{0.504}} & \textcolor{tabG}{0.505} & \textcolor{tabG}{0.511} & \textcolor{tabG}{0.510} & \textcolor{tabG}{0.505} & \textbf{\textcolor{tabG}{0.501}} \\
    \textbf{EuroSAT} & 0.514 & \textcolor{tabG}{\underline{0.503}} & \textcolor{tabR}{0.516} & \textcolor{tabG}{0.508} & \textcolor{tabG}{0.508} & \textcolor{tabR}{0.532} & \textbf{\textcolor{tabG}{0.502}} & \textbf{\textcolor{tabG}{0.502}}\\
    \textbf{TinyImagenet} & 0.509 & \textcolor{tabG}{0.506} & \textcolor{tabG}{0.504} & \textcolor{tabR}{0.530} & \textcolor{tabR}{0.544} & \textcolor{tabR}{0.520} & \textcolor{tabG}{\underline{0.502}} & \textbf{\textcolor{tabG}{0.501}} \\
    \textbf{OxfordFlowers} & 0.556 & \textcolor{tabR}{0.595} & \textcolor{tabR}{0.877} & \textcolor{tabR}{0.677} & \textcolor{tabR}{0.589} & \textcolor{tabR}{0.590} & \textbf{\textcolor{tabG}{0.529}} & \textcolor{tabG}{\underline{0.535}}\\
    \textbf{STL-10} & 0.522 & \textcolor{tabG}{0.508} & \textcolor{tabG}{0.521} & \textcolor{tabG}{0.513} & \textbf{\textcolor{tabG}{0.501}} & \textcolor{tabG}{0.505} & \textcolor{tabG}{\underline{0.503}} & \textcolor{tabG}{0.504}\\
    \textbf{Cinic-10} & 0.508 & \textcolor{tabR}{0.534} & \textcolor{tabG}{\underline{0.505}} & \textbf{\textcolor{tabG}{0.501}} & \textbf{\textcolor{tabG}{0.501}} & \textbf{\textcolor{tabG}{0.501}} & \textbf{\textcolor{tabG}{0.501}} & \textbf{\textcolor{tabG}{0.501}}\\
    \hline
    \textbf{Average} & 0.523 & \textcolor{tabR}{0.529} & \textcolor{tabR}{0.555} & \textcolor{tabR}{0.532} & \textcolor{tabG}{\underline{0.521}} & \textcolor{tabG}{0.522} & \textbf{\textcolor{tabG}{0.507}} & \textbf{\textcolor{tabG}{0.507}}\\
    \hline
    \end{tabularx}}%
    \label{table:ok}
\end{table}

% \newpage
% \section*{Training Time}
% \input{tabs/time}
